# Supplementary material for: Minimax Lower Bounds for Transfer Learning with Linear and One-hidden Layer Neural Networks
Source: arXiv:2006.10581 source file (2020-06-16)
Supplement: Supplementary file 1 [file supp.tex]

\section*{Road Map of Supplementary}
The first eight pages of the supplementary are essentially the same as the main submission except for an enhanced numerical section in \ref{numresults} which contains some additional simulations. \textcolor{red}{We also note that Definition 4 of the main submission contained a typo which we have fixed in this supplementary}. This supplementary also includes a proof sketch in Section \ref{sketch} and all of the proofs of the main results in Appendix \ref{appendix}.
